# Supplementary material for: ACTT: Automotive CAN Tokenization and Translation
Source: arXiv:1811.07897 source file (2018-11-19)
Supplement: Supplementary file 1 [file 99-appendix.tex]

\section*{Appendix}
\addcontentsline{toc}{section}{Appendix}
\label{app:appendix}

%% to reference this section use \hyperref[app:appendix]{Appendix}
